# Supplementary material for: A Bandit Approach to Maximum Inner Product Search
Source: arXiv:1812.06360 source file (2018-12-15)
Supplement: Supplementary file 1 [file supplement.tex]

\relax
%File: formatting-instruction.tex
\documentclass[letterpaper]{article}
\usepackage{aaai19}
\usepackage{times}
\usepackage{helvet}
\usepackage{courier}
\usepackage{url}  %Required
\usepackage{graphicx}
\frenchspacing  %Required
\setlength{\pdfpagewidth}{8.5in}  %Required
\setlength{\pdfpageheight}{11in}  %Required

\usepackage[table,xcdraw]{xcolor}
\usepackage{algorithm}
\usepackage{algorithmic}

\usepackage{amssymb}
\usepackage{amsmath}
\usepackage{amsthm}
\usepackage[toc,title]{appendix}
\usepackage{bm}
\usepackage{color}
\usepackage{fancyhdr}
\usepackage[acronym,shortcuts,nonumberlist]{glossaries}

\usepackage{multirow}
\usepackage{comment}

\newcommand{\ignore}[1]{}
 % ---}

%\renewcommand{\cancut}[1]{\textcolor{blue}{}}
\newcommand{\tempcut}[1]{}

\definecolor{mypink3}{cmyk}{0, 0.7808, 0.4429, 0.1412}
% other colors:  magenta, orange, brown, mypink3

% hyperref makes hyperlinks in the resulting PDF.
% If your build breaks (sometimes temporarily if a hyperlink spans a page)
% please comment out the following usepackage line and replace
% \usepackage{icml2018} with \usepackage[nohyperref]{icml2018} above.
%\usepackage{hyperref}

% Attempt to make hyperref and algorithmic work together better:

\title{Supplement to ``A Bandit Approach  to Maximum Inner Product Search"}

\begin{document}
%\date{}
%\maketitle

\input{supplement_proof}

%\setcitestyle{square, comma, numbers,sort&compress, super}
\bibliographystyle{aaai}
\bibliography{mips}
\pagenumbering{gobble}

\end{document}
